# Supplementary material for: Discovery of Standstills in the SU UMa-Type Dwarf Nova NY Serpentis
Source: arXiv:1901.05100 ancillary file (2019-01-16)
Supplement: Supplementary file 1 [file si.pdf]

Publ. Astron. Soc. Japan (2014) 00(0), 1–14
doi: 10.1093/pasj/xxx000


# Supplementary Infomation to Discovery of Standstills in the SU UMa-Type Dwarf Nova NY Serpentis

**T. Kato et al.**

Received ; Accepted

## Abstract

This is Supplementary Infomation to Discovery of Standstills in the SU UMa-Type Dwarf Nova NY Serpentis (online only)

## E-section 1 Data analysis

The data analysis was performed in the same way described in Kato et al. (2009) and Kato et al. (2014) and we used R software[1] for data analysis.

In de-trending the data, we used locally-weighted polynomial regression (LOWESS: Cleveland 1979). The times of superhumps maxima were determined by the template fitting method as described in Kato et al. (2009). The times of all observations are expressed in barycentric Julian days (BJD).

We used phase dispersion minimization (PDM; Stellingwerf 1978) for period analysis and $1\sigma$ errors for the PDM analysis was estimated by the methods of Fernie (1989) and Kato et al. (2010).

## E-section 2 Superhump excess and disk radius

This part is an excerpt from Kato and Osaki (2013). The dynamical precession rate is a function of the disk radius and the mass ratio, and observing the dynamical precession rate ($\epsilon^*$ in the text), we can determine the mass ratio from the disk radius and vice versa.

The dynamical precession rate, $\omega_{\rm dyn}(\omega_{\rm dyn}/\omega_{\rm orb}= \epsilon^*$, when the pressure effect can be neglected) at radius $r$ in the disk can be expressed by

$$\omega_{\rm dyn}/\omega_{\rm orb} = \frac{q}{\sqrt{1+q}}\left[\frac{1}{4}\frac{1}{\sqrt{r}}\frac{d}{dr}\left(r^2\frac{db^{(0)}_{1/2}}{dr}\right)\right] = \frac{q}{\sqrt{1+q}}\left[\frac{1}{4}\sqrt{r}b^{(1)}_{3/2}\right]. \quad \text{(E1)}$$

where $r$ is the dimensionless radius measured in units of the binary separation $A$, $\omega_{\rm orb}$ is the angular frequency of the binary motion, and $\frac{1}{2}b^{(j)}_{s/2}$ is the Laplace coefficient

$$\frac{1}{2}b^{(j)}_{s/2}(r) = \frac{1}{2\pi}\int_0^{2\pi}\frac{\cos(j\phi)d\phi}{(1+r^2-2r\cos\phi)^{s/2}}, \quad \text{(E2)}$$

respectively.

[1] The R Foundation for Statistical Computing: <http://cran.r-project.org/>.

© 2014. Astronomical Society of Japan.

## References

Cleveland, W. S. 1979, J. Amer. Statist. Assoc., 74, 829
Fernie, J. D. 1989, PASP, 101, 225
Kato, T., et al. 2014, PASJ, 66, 90
Kato, T., et al. 2009, PASJ, 61, S395
Kato, T., et al. 2010, PASJ, 62, 1525
Kato, T., & Osaki, Y. 2013, PASJ, 65, 115
Osaki, Y., & Kato, T. 2013a, PASJ, 65, 50
Osaki, Y., & Kato, T. 2013b, PASJ, 65, 95
Stellingwerf, R. F. 1978, ApJ, 224, 953

**E-table 1.** Log of Observations

| Start* | End* | Mean mag | error | $N^{\dagger}$ | Observer‡ | Filter |
|---|---|---|---|---|---|---|
| 58172.2051 | 58172.3539 | 0.178 | 0.007 | 62 | KU1 | Ic |
| 58172.3470 | 58172.3650 | 1.809 | 0.003 | 25 | OKU | C |
| 58172.4283 | 58172.6312 | 15.224 | 0.004 | 75 | Skl | C |
| 58173.1422 | 58173.3660 | 0.134 | 0.004 | 283 | KU1 | Ic |
| 58173.1464 | 58173.3629 | 1.832 | 0.001 | 289 | OKU | C |
| 58176.1463 | 58176.3650 | 1.837 | 0.001 | 292 | OKU | C |
| 58176.1617 | 58176.3192 | 0.159 | 0.003 | 212 | KU1 | Ic |
| 58177.1520 | 58177.3648 | 1.782 | 0.001 | 285 | OKU | C |
| 58177.1589 | 58177.3626 | 0.118 | 0.006 | 225 | KU1 | Ic |
| 58179.2626 | 58179.3585 | 1.863 | 0.002 | 129 | OKU | C |
| 58180.1488 | 58180.3579 | 1.839 | 0.002 | 278 | OKU | C |
| 58181.1353 | 58181.3563 | 1.813 | 0.002 | 295 | OKU | C |
| 58183.4633 | 58183.5174 | 15.466 | 0.003 | 74 | CRI | C |
| 58184.1627 | 58184.3455 | 1.844 | 0.001 | 241 | OKU | C |
| 58185.4194 | 58185.5209 | 15.413 | 0.002 | 138 | CRI | C |
| 58187.4367 | 58187.5810 | 15.906 | 0.005 | 63 | BSM | C |
| 58188.1362 | 58188.3521 | 1.856 | 0.001 | 286 | OKU | C |
| 58188.1567 | 58188.1926 | -0.202 | 0.004 | 49 | KU1 | C |
| 58189.0737 | 58189.3176 | -0.186 | 0.003 | 324 | KU1 | C |
| 58189.1544 | 58189.3482 | 1.828 | 0.001 | 260 | OKU | C |
| 58189.4367 | 58189.6208 | 15.431 | 0.002 | 412 | CRI | C |
| 58190.1614 | 58190.3537 | -0.224 | 0.003 | 257 | KU1 | C |
| 58190.1666 | 58190.3493 | 1.808 | 0.002 | 244 | OKU | C |
| 58191.1314 | 58191.3442 | 1.848 | 0.001 | 283 | OKU | C |
| 58191.1503 | 58191.3425 | -0.171 | 0.004 | 130 | KU1 | C |
| 58191.3731 | 58191.4631 | 15.322 | 0.011 | 17 | Skl | C |
| 58192.1289 | 58192.3424 | 1.896 | 0.002 | 276 | OKU | C |
| 58193.3988 | 58193.5967 | 15.412 | 0.001 | 268 | CRI | C |
| 58194.2151 | 58194.3342 | 1.752 | 0.002 | 160 | OKU | C |
| 58194.3673 | 58194.4036 | 15.410 | 0.004 | 50 | CRI | C |
| 58194.4061 | 58194.4200 | 15.153 | 0.010 | 7 | Skl | C |
| 58195.1283 | 58195.3449 | 1.781 | 0.001 | 288 | OKU | C |
| 58200.2597 | 58200.2994 | 1.008 | 0.001 | 54 | OKU | C |
| 58200.4858 | 58200.6102 | 14.688 | 0.005 | 116 | Lis | R |
| 58201.1275 | 58201.3317 | 1.042 | 0.003 | 509 | OKU | C |
| 58201.4211 | 58201.5890 | -1.038 | 0.003 | 217 | DPV | C |
| 58201.4781 | 58201.5910 | 14.709 | 0.005 | 260 | Lis | R |
| 58202.1394 | 58202.3334 | 1.195 | 0.003 | 260 | OKU | C |
| 58202.1498 | 58202.2489 | -0.841 | 0.004 | 134 | KU1 | C |
| 58202.3831 | 58202.4990 | 14.833 | 0.004 | 211 | Lis | R |
| 58202.3980 | 58202.6087 | -0.911 | 0.003 | 271 | DPV | C |
| 58203.1304 | 58203.3355 | 1.242 | 0.003 | 187 | OKU | C |
| 58203.3256 | 58203.5027 | 14.880 | 0.002 | 240 | CRI | C |
| 58203.3739 | 58203.4470 | -0.813 | 0.003 | 93 | DPV | C |
| 58203.6130 | 58203.6347 | 15.030 | 0.005 | 27 | RPc | C |
| 58203.7490 | 58203.9045 | 15.186 | 0.004 | 130 | MZK | C |

*BJD−2400000

†Number of observations.

‡Observer's code (observations with magnitude larger than 10 reported real magnitudes and others reported differential ones): BSM (S. Brincat), CRI, CR2 (Crimean Astrophys. Obs), DKS (S. Dvorak), DPV (P. Dubovsky), IMi (I. Miller), KU1 (Kyoto U.), Kai (K. Kasai), Kaz (Kazan' Obs.), Lis (Lisnyky Obs.), MZK (K. Menzies), May (Mayaki Obs.), OKU (Osaka Kyoiku U.), RPc (R. Pickard), Skl (A. Sklyanov), Ter (Terskol Obs.), deM (E. de Miguel), BJA is an AAVSO observer,

**E-table 1.** Log of Observations (continued)

| Start* | End* | Mean mag | error | $N^\dagger$ | Observer‡ | Filter |
|---|---|---|---|---|---|---|
| 58204.1323 | 58204.3353 | 1.342 | 0.002 | 272 | OKU | C |
| 58205.1256 | 58205.3346 | 1.431 | 0.002 | 280 | OKU | C |
| 58206.1151 | 58206.3355 | 1.536 | 0.002 | 294 | OKU | C |
| 58206.1552 | 58206.2880 | -0.468 | 0.004 | 179 | KU1 | C |
| 58207.3303 | 58207.5282 | 15.273 | 0.003 | 268 | CRI | C |
| 58208.1273 | 58208.3341 | 1.802 | 0.002 | 277 | OKU | C |
| 58208.3083 | 58208.4479 | 15.445 | 0.003 | 179 | CRI | C |
| 58209.1572 | 58209.3288 | 2.215 | 0.006 | 229 | OKU | C |
| 58209.3750 | 58209.5436 | 15.733 | 0.008 | 73 | Skl | C |
| 58212.1275 | 58212.3246 | 2.208 | 0.004 | 264 | OKU | C |
| 58212.3886 | 58212.4894 | 15.854 | 0.004 | 134 | CRI | C |
| 58213.3860 | 58213.5098 | 16.407 | 0.007 | 168 | CRI | C |
| 58214.2959 | 58214.5247 | 16.567 | 0.014 | 99 | Skl | C |
| 58214.3374 | 58214.4696 | 16.671 | 0.009 | 68 | CRI | C |
| 58215.2862 | 58215.4658 | 16.747 | 0.008 | 125 | CRI | C |
| 58215.7823 | 58215.9336 | 16.925 | 0.007 | 185 | BJA | C |
| 58216.2976 | 58216.4209 | 15.411 | 0.002 | 167 | CRI | C |
| 58216.4561 | 58216.4670 | -0.342 | 0.006 | 15 | DPV | C |
| 58217.2768 | 58217.4324 | 15.505 | 0.002 | 209 | CRI | C |
| 58217.4087 | 58217.5775 | -0.105 | 0.003 | 216 | DPV | C |
| 58217.4558 | 58217.5421 | 15.519 | 0.004 | 34 | May | R |
| 58218.2473 | 58218.5201 | 15.874 | 0.004 | 119 | Skl | C |
| 58218.2907 | 58218.4557 | 16.038 | 0.003 | 218 | CRI | C |
| 58218.3249 | 58218.5753 | 0.438 | 0.006 | 320 | DPV | C |
| 58218.4192 | 58218.4811 | 16.022 | 0.005 | 27 | May | R |
| 58218.4261 | 58218.5580 | 16.006 | 0.005 | 267 | Ter | C |
| 58219.2892 | 58219.5181 | 16.522 | 0.006 | 100 | Skl | C |
| 58219.3815 | 58219.4670 | 16.608 | 0.005 | 36 | May | R |
| 58219.4056 | 58219.5300 | 16.586 | 0.005 | 316 | Ter | C |
| 58220.1261 | 58220.1305 | 3.203 | 0.015 | 5 | OKU | C |
| 58220.2801 | 58220.4182 | 16.615 | 0.008 | 186 | CRI | C |
| 58221.4252 | 58221.5904 | 16.429 | 0.008 | 224 | CRI | C |
| 58222.3770 | 58222.4874 | 15.377 | 0.002 | 150 | CRI | C |
| 58223.3931 | 58223.5257 | 15.417 | 0.003 | 178 | CRI | C |
| 58224.0886 | 58224.1013 | 2.164 | 0.010 | 13 | OKU | C |
| 58224.3895 | 58224.4770 | 15.954 | 0.004 | 119 | CRI | C |
| 58224.4474 | 58224.5008 | 15.913 | 0.004 | 123 | Ter | C |
| 58225.4717 | 58225.5272 | 16.745 | 0.006 | 118 | Ter | C |
| 58226.4063 | 58226.5534 | 16.913 | 0.009 | 214 | Ter | C |
| 58226.7111 | 58226.9098 | 17.288 | 0.009 | 137 | DKS | C |
| 58227.1077 | 58227.3093 | 3.285 | 0.005 | 207 | OKU | C |
| 58227.2972 | 58227.5502 | 1.198 | 0.007 | 169 | DPV | C |
| 58227.4402 | 58227.5476 | 17.137 | 0.007 | 117 | deM | C |
| 58228.2954 | 58228.5958 | 0.977 | 0.008 | 173 | DPV | C |
| 58228.7199 | 58228.9029 | 16.129 | 0.017 | 122 | DKS | C |
| 58228.7620 | 58228.9167 | 16.180 | 0.012 | 240 | BJA | C |
| 58229.1071 | 58229.3004 | 1.634 | 0.001 | 207 | OKU | C |
| 58229.2983 | 58229.5882 | -0.552 | 0.002 | 184 | DPV | C |
| 58229.3822 | 58229.4170 | 15.147 | 0.009 | 39 | CRI | C |
| 58230.1012 | 58230.3050 | 1.793 | 0.003 | 214 | OKU | C |
| 58230.2953 | 58230.4883 | -0.228 | 0.003 | 229 | DPV | C |
| 58230.3927 | 58230.5162 | 15.496 | 0.004 | 59 | CRI | C |
| 58231.1971 | 58231.3050 | 2.434 | 0.005 | 144 | OKU | C |
| 58231.3064 | 58231.5842 | 0.532 | 0.004 | 187 | DPV | C |
| 58231.3906 | 58231.5162 | 16.205 | 0.004 | 60 | CRI | C |

**E-table 1.** Log of Observations (continued)

| Start* | End* | Mean mag | error | $N^{\dagger}$ | Observer‡ | Filter |
|---|---|---|---|---|---|---|
| 58231.7628 | 58231.9134 | 16.924 | 0.005 | 200 | BJA | C |
| 58232.4840 | 58232.5730 | 16.928 | 0.013 | 43 | CRI | C |
| 58233.4613 | 58233.5614 | 16.990 | 0.010 | 48 | CRI | C |
| 58235.4651 | 58235.5696 | 16.532 | 0.007 | 50 | CRI | C |
| 58236.0765 | 58236.3033 | 1.594 | 0.003 | 212 | OKU | C |
| 58236.3325 | 58236.3410 | 15.100 | 0.013 | 5 | CRI | C |
| 58237.0971 | 58237.3024 | 1.678 | 0.002 | 247 | OKU | C |
| 58237.3537 | 58237.3666 | 15.354 | 0.008 | 10 | CRI | C |
| 58237.7677 | 58237.9134 | 15.946 | 0.003 | 227 | BJA | C |
| 58238.0997 | 58238.2279 | 2.147 | 0.005 | 115 | OKU | C |
| 58238.3099 | 58238.3530 | 15.932 | 0.008 | 31 | CRI | C |
| 58239.1066 | 58239.3026 | 3.021 | 0.008 | 135 | OKU | C |
| 58239.3985 | 58239.4114 | 16.893 | 0.018 | 10 | CRI | C |
| 58242.1198 | 58242.2893 | 3.222 | 0.008 | 79 | OKU | C |
| 58242.3045 | 58242.4558 | 1.111 | 0.006 | 102 | DPV | C |
| 58243.0988 | 58243.2929 | 1.590 | 0.002 | 260 | OKU | C |
| 58243.3453 | 58243.4951 | -0.621 | 0.002 | 93 | DPV | C |
| 58244.1333 | 58244.2882 | 1.594 | 0.002 | 208 | OKU | C |
| 58244.3633 | 58244.5028 | -0.413 | 0.002 | 95 | DPV | C |
| 58245.3187 | 58245.4983 | 0.129 | 0.005 | 118 | DPV | C |
| 58248.0703 | 58248.1571 | 3.542 | 0.008 | 112 | OKU | C |
| 58249.0985 | 58249.2557 | 3.179 | 0.005 | 208 | OKU | C |
| 58250.3174 | 58250.5338 | -0.656 | 0.003 | 248 | DPV | C |
| 58251.1369 | 58251.1511 | 1.482 | 0.008 | 18 | OKU | C |
| 58251.3058 | 58251.3505 | 14.997 | 0.010 | 35 | CRI | C |
| 58251.3092 | 58251.4069 | -0.587 | 0.002 | 124 | DPV | C |
| 58252.2845 | 58252.4735 | 15.471 | 0.004 | 89 | CRI | C |
| 58252.3133 | 58252.3652 | -0.122 | 0.004 | 36 | DPV | C |
| 58253.1015 | 58253.2611 | 2.535 | 0.005 | 211 | OKU | C |
| 58253.3344 | 58253.5356 | 16.216 | 0.006 | 96 | CRI | C |
| 58254.2616 | 58254.3781 | 16.939 | 0.013 | 56 | CRI | C |
| 58255.2189 | 58255.2338 | 3.472 | 0.014 | 20 | OKU | C |
| 58255.2776 | 58255.3982 | 16.856 | 0.023 | 49 | CRI | C |
| 58256.1141 | 58256.2759 | 3.378 | 0.007 | 202 | OKU | C |
| 58257.3256 | 58257.4817 | 16.489 | 0.005 | 146 | CRI | C |
| 58258.2986 | 58258.3927 | 14.772 | 0.002 | 88 | CRI | C |
| 58259.3123 | 58259.3974 | 14.949 | 0.002 | 77 | CRI | C |
| 58260.1281 | 58260.1992 | 1.634 | 0.003 | 93 | OKU | C |
| 58260.4625 | 58260.4655 | 15.273 | 0.006 | 5 | CRI | C |
| 58261.2949 | 58261.3482 | 15.459 | 0.001 | 72 | CRI | C |
| 58262.3032 | 58262.3099 | 15.624 | 0.005 | 10 | CRI | C |
| 58263.2911 | 58263.2978 | 15.530 | 0.004 | 9 | CRI | C |
| 58264.3006 | 58264.3073 | 15.475 | 0.008 | 10 | CRI | C |
| 58264.9933 | 58265.2811 | 1.978 | 0.003 | 152 | OKU | C |
| 58265.2734 | 58265.2949 | 15.602 | 0.006 | 30 | CRI | C |
| 58266.2898 | 58266.2965 | 15.515 | 0.007 | 9 | CRI | C |
| 58268.2774 | 58268.2841 | 15.556 | 0.009 | 10 | CRI | C |
| 58269.3288 | 58269.3354 | 15.590 | 0.009 | 10 | CRI | C |
| 58270.3237 | 58270.3304 | 15.533 | 0.005 | 10 | CRI | C |
| 58270.9950 | 58271.0018 | 1.819 | 0.005 | 10 | OKU | C |
| 58271.2986 | 58271.3053 | 15.476 | 0.003 | 10 | CRI | C |
| 58271.9827 | 58271.9887 | 1.923 | 0.010 | 8 | OKU | C |
| 58272.3071 | 58272.3137 | 15.611 | 0.007 | 10 | CRI | C |
| 58273.2938 | 58273.3042 | 15.636 | 0.003 | 15 | CRI | C |
| 58273.9936 | 58273.9996 | 1.887 | 0.011 | 8 | OKU | C |

**E-table 1.** Log of Observations (continued)

| Start* | End* | Mean mag | error | $N^{\dagger}$ | Observer‡ | Filter |
|---|---|---|---|---|---|---|
| 58274.2844 | 58274.2948 | 15.446 | 0.006 | 15 | CRI | C |
| 58275.2991 | 58275.5153 | 15.422 | 0.006 | 190 | CRI | C |
| 58276.3176 | 58276.5013 | 15.558 | 0.002 | 249 | CRI | C |
| 58277.1142 | 58277.1209 | 1.928 | 0.006 | 10 | OKU | C |
| 58277.3583 | 58277.4324 | 15.530 | 0.002 | 101 | CRI | C |
| 58278.3138 | 58278.5354 | 15.536 | 0.001 | 1096 | CRI | C |
| 58278.9976 | 58279.0074 | 1.935 | 0.007 | 10 | OKU | C |
| 58279.3016 | 58279.4402 | 15.595 | 0.001 | 607 | CRI | C |
| 58280.3021 | 58280.5096 | 15.426 | 0.004 | 99 | CRI | C |
| 58281.3092 | 58281.5233 | 15.341 | 0.002 | 100 | CRI | C |
| 58282.1849 | 58282.1909 | 1.917 | 0.005 | 9 | OKU | C |
| 58282.3588 | 58282.5158 | -0.116 | 0.003 | 147 | CR2 | C |
| 58284.3160 | 58284.5152 | 15.348 | 0.003 | 87 | CRI | C |
| 58284.3260 | 58284.4916 | 15.277 | 0.003 | 99 | Skl | C |
| 58285.9986 | 58286.0053 | 1.870 | 0.004 | 10 | OKU | C |
| 58289.3102 | 58289.5219 | 15.449 | 0.002 | 101 | CRI | C |
| 58290.2991 | 58290.4579 | 15.347 | 0.004 | 75 | CRI | C |
| 58291.2984 | 58291.4441 | 15.297 | 0.003 | 88 | Skl | C |
| 58291.9937 | 58291.9991 | 1.922 | 0.013 | 4 | OKU | C |
| 58294.3176 | 58294.4531 | 15.406 | 0.004 | 65 | CRI | C |
| 58298.1535 | 58298.1595 | 2.049 | 0.011 | 9 | OKU | C |
| 58300.3142 | 58300.4324 | 15.307 | 0.005 | 67 | Skl | C |
| 58300.9807 | 58300.9874 | 1.940 | 0.007 | 10 | OKU | C |
| 58301.9666 | 58301.9719 | 1.955 | 0.009 | 7 | OKU | C |
| 58302.2875 | 58302.3746 | 15.504 | 0.002 | 118 | CRI | C |
| 58303.3006 | 58303.4688 | 15.484 | 0.002 | 228 | CRI | C |
| 58304.2886 | 58304.4034 | 15.492 | 0.002 | 156 | CRI | C |
| 58305.2899 | 58305.4270 | 15.608 | 0.002 | 169 | CRI | C |
| 58308.1017 | 58308.1069 | 1.800 | 0.009 | 8 | OKU | C |
| 58309.1546 | 58309.1622 | 1.914 | 0.006 | 7 | OKU | C |
| 58309.2954 | 58309.3021 | 15.514 | 0.005 | 10 | CRI | C |
| 58310.3594 | 58310.4919 | 15.680 | 0.006 | 190 | Skl | C |
| 58311.2958 | 58311.3023 | 15.581 | 0.004 | 10 | CRI | C |
| 58311.3655 | 58311.5411 | 15.817 | 0.003 | 241 | Kai | C |
| 58312.2818 | 58312.4041 | 15.417 | 0.003 | 164 | CRI | C |
| 58312.3709 | 58312.5367 | 15.672 | 0.003 | 221 | Kai | C |
| 58313.2799 | 58313.4015 | 15.163 | 0.002 | 163 | CRI | C |
| 58313.9593 | 58313.9653 | 1.204 | 0.007 | 9 | OKU | C |
| 58314.3804 | 58314.4697 | 14.537 | 0.009 | 114 | CRI | C |
| 58314.9607 | 58314.9667 | 0.825 | 0.010 | 6 | OKU | C |
| 58315.3584 | 58315.4278 | 14.618 | 0.010 | 68 | CRI | C |
| 58315.9782 | 58316.0466 | 1.001 | 0.012 | 36 | OKU | C |
| 58316.3934 | 58316.4119 | 14.545 | 0.013 | 9 | Skl | C |
| 58317.0611 | 58317.0739 | 1.136 | 0.015 | 15 | OKU | C |
| 58318.0563 | 58318.1379 | 1.155 | 0.004 | 102 | OKU | C |
| 58318.4187 | 58318.5148 | 14.887 | 0.004 | 130 | IMi | C |
| 58318.9691 | 58319.0545 | 1.250 | 0.004 | 115 | OKU | C |
| 58319.3349 | 58319.3488 | 14.728 | 0.008 | 40 | CRI | C |
| 58319.4164 | 58319.5289 | 14.964 | 0.003 | 148 | IMi | C |
| 58320.9690 | 58321.1247 | 1.428 | 0.004 | 140 | OKU | C |
| 58321.2681 | 58321.4104 | 15.072 | 0.003 | 191 | CRI | C |
| 58321.9992 | 58322.0059 | 1.470 | 0.006 | 10 | OKU | C |
| 58322.2650 | 58322.3718 | 15.200 | 0.002 | 142 | CRI | C |
| 58322.4103 | 58322.5146 | 15.279 | 0.004 | 137 | IMi | C |
| 58323.0696 | 58323.0748 | 1.702 | 0.007 | 7 | OKU | C |
| 58323.9558 | 58323.9618 | 1.735 | 0.010 | 9 | OKU | C |

**E-table 1.** Log of Observations (continued)

| Start* | End* | Mean mag | error | $N^{\dagger}$ | Observer‡ | Filter |
|---|---|---|---|---|---|---|
| 58325.3120 | 58325.3616 | 15.769 | 0.005 | 67 | CRI | C |
| 58325.4044 | 58325.5102 | 15.943 | 0.009 | 138 | IMi | C |
| 58326.2640 | 58326.4234 | 15.935 | 0.004 | 215 | CRI | C |
| 58328.2703 | 58328.3666 | 15.933 | 0.005 | 131 | CRI | C |
| 58328.9539 | 58328.9599 | 2.475 | 0.013 | 8 | OKU | C |
| 58329.9896 | 58329.9963 | 2.478 | 0.009 | 9 | OKU | C |
| 58330.3185 | 58330.4426 | 16.119 | 0.005 | 162 | CRI | C |
| 58330.9562 | 58330.9622 | 2.204 | 0.015 | 9 | OKU | C |
| 58331.3682 | 58331.3799 | 15.589 | 0.016 | 10 | Lis | R |
| 58331.9574 | 58331.9626 | 2.092 | 0.006 | 8 | OKU | C |
| 58332.2936 | 58332.4055 | 15.894 | 0.005 | 151 | CRI | C |
| 58332.9719 | 58332.9779 | 2.622 | 0.017 | 9 | OKU | C |
| 58333.3349 | 58333.3416 | 16.300 | 0.013 | 20 | Lis | R |
| 58333.9565 | 58333.9652 | 3.131 | 0.017 | 9 | OKU | C |
| 58334.3220 | 58334.3358 | 16.486 | 0.009 | 20 | CRI | C |
| 58334.3343 | 58334.3676 | 16.558 | 0.008 | 95 | Lis | R |
| 58334.9697 | 58335.1105 | 2.719 | 0.006 | 174 | OKU | C |
| 58335.3276 | 58335.3416 | 16.170 | 0.019 | 20 | CRI | C |
| 58335.4095 | 58335.4145 | 15.950 | 0.024 | 15 | Lis | R |
| 58335.9866 | 58336.0952 | 2.427 | 0.008 | 107 | OKU | C |
| 58336.2533 | 58336.2671 | 15.697 | 0.012 | 20 | CRI | C |
| 58336.3361 | 58336.3713 | 15.619 | 0.008 | 88 | Lis | R |
| 58336.9650 | 58337.0092 | 1.917 | 0.004 | 39 | OKU | C |
| 58337.2667 | 58337.4034 | 15.593 | 0.003 | 150 | CRI | C |
| 58337.9793 | 58338.0684 | 2.320 | 0.006 | 120 | OKU | C |
| 58338.2660 | 58338.3898 | 16.074 | 0.006 | 168 | CRI | C |
| 58339.2657 | 58339.4063 | 16.656 | 0.014 | 67 | CRI | C |
| 58339.3467 | 58339.4127 | 16.531 | 0.014 | 187 | Lis | R |
| 58340.2955 | 58340.3658 | 16.791 | 0.013 | 34 | CRI | C |
| 58340.3218 | 58340.4370 | 16.771 | 0.009 | 260 | Lis | R |
| 58340.9989 | 58341.0760 | 3.354 | 0.009 | 95 | OKU | C |
| 58341.4061 | 58341.4177 | 16.336 | 0.026 | 10 | Ter | R |
| 58342.0258 | 58342.0345 | 2.479 | 0.022 | 7 | OKU | C |
| 58342.2753 | 58342.3851 | 15.883 | 0.003 | 198 | Ter | R |
| 58342.9721 | 58342.9765 | 2.341 | 0.013 | 4 | OKU | C |
| 58344.0256 | 58344.0286 | 2.012 | 0.025 | 5 | OKU | C |
| 58344.2673 | 58344.2758 | 15.514 | 0.004 | 5 | CRI | C |
| 58345.2629 | 58345.2715 | 15.776 | 0.003 | 5 | CRI | C |
| 58345.3027 | 58345.3914 | 15.698 | 0.003 | 251 | Lis | R |
| 58346.2643 | 58346.2729 | 16.438 | 0.013 | 5 | CRI | C |
| 58346.3826 | 58346.3909 | 16.409 | 0.020 | 20 | Ter | C |
| 58347.2568 | 58347.2651 | 16.722 | 0.020 | 20 | Ter | C |
| 58347.2661 | 58347.2746 | 16.761 | 0.017 | 5 | CRI | C |
| 58347.9578 | 58347.9666 | 3.485 | 0.016 | 9 | OKU | C |
| 58348.2676 | 58348.2761 | 17.009 | 0.016 | 5 | CRI | C |
| 58348.9662 | 58348.9750 | 3.562 | 0.011 | 7 | OKU | C |
| 58349.2782 | 58349.2867 | 17.053 | 0.019 | 5 | CRI | C |
| 58349.9419 | 58349.9507 | 3.403 | 0.021 | 8 | OKU | C |
| 58350.2716 | 58350.2801 | 16.394 | 0.013 | 5 | CRI | C |
| 58351.2637 | 58351.2722 | 15.891 | 0.007 | 5 | CRI | C |
| 58351.3298 | 58351.3298 | 15.714 | – | 1 | Lis | R |
| 58352.2740 | 58352.2825 | 15.464 | 0.006 | 5 | CRI | C |
| 58353.2649 | 58353.2734 | 15.442 | 0.008 | 5 | CRI | C |
| 58354.2710 | 58354.2795 | 16.108 | 0.010 | 5 | CRI | C |
| 58354.3214 | 58354.3214 | 15.841 | – | 1 | Lis | R |

**E-table 1.** Log of Observations (continued)

| Start* | End* | Mean mag | error | $N^\dagger$ | Observer‡ | Filter |
|---|---|---|---|---|---|---|
| 58355.2651 | 58355.2736 | 16.676 | 0.008 | 5 | CRI | C |
| 58355.3269 | 58355.3269 | 16.803 | – | 1 | Lis | R |
| 58355.9409 | 58355.9486 | 3.109 | 0.017 | 8 | OKU | C |
| 58357.3528 | 58357.3556 | 16.528 | 0.115 | 5 | Lis | R |
| 58357.9322 | 58357.9409 | 3.371 | 0.034 | 9 | OKU | C |
| 58358.2569 | 58358.2654 | 16.635 | 0.017 | 5 | CRI | C |
| 58358.9382 | 58358.9404 | 2.596 | 0.020 | 3 | OKU | C |
| 58359.9350 | 58359.9438 | 2.310 | 0.008 | 9 | OKU | C |
| 58360.9441 | 58360.9507 | 2.534 | 0.016 | 7 | OKU | C |
| 58361.2669 | 58361.2754 | 16.272 | 0.026 | 5 | CRI | C |
| 58361.3252 | 58361.3308 | 16.533 | 0.029 | 6 | Lis | R |
| 58362.2570 | 58362.2655 | 16.710 | 0.013 | 5 | CRI | C |
| 58363.2494 | 58363.2579 | 17.025 | 0.019 | 5 | CRI | C |
| 58364.2455 | 58364.2609 | 16.625 | 0.014 | 5 | CRI | C |
| 58365.2524 | 58365.3312 | 16.258 | 0.004 | 35 | CRI | C |
| 58366.2468 | 58366.3085 | 16.575 | 0.009 | 30 | CRI | C |
| 58366.9529 | 58366.9551 | 3.163 | 0.029 | 3 | OKU | C |
| 58369.2620 | 58369.3153 | 17.074 | 0.013 | 26 | CRI | C |
| 58374.2244 | 58374.2799 | 16.329 | 0.013 | 74 | Lis | R |
| 58379.2559 | 58379.2858 | 16.957 | 0.043 | 15 | CRI | C |
| 58380.2026 | 58380.2196 | 17.183 | 0.033 | 7 | CRI | C |
| 58381.2051 | 58381.2179 | 15.368 | 0.004 | 7 | CRI | C |
| 58382.2022 | 58382.2150 | 15.259 | 0.011 | 7 | CRI | C |
| 58383.2280 | 58383.2366 | 15.850 | 0.009 | 5 | CRI | C |
| 58388.1970 | 58388.2056 | 17.066 | 0.025 | 5 | CRI | C |
| 58389.2006 | 58389.2092 | 16.888 | 0.022 | 5 | CRI | C |
| 58390.1873 | 58390.2001 | 16.533 | 0.028 | 7 | CRI | C |
| 58397.2029 | 58397.2114 | 17.117 | 0.021 | 5 | CRI | C |
| 58400.2240 | 58400.2326 | 17.330 | 0.046 | 5 | CRI | C |
| 58403.1823 | 58403.1942 | 14.832 | 0.005 | 17 | CRI | C |
| 58404.2002 | 58404.2088 | 14.738 | 0.019 | 5 | CRI | C |
| 58405.2552 | 58405.2916 | 14.849 | 0.012 | 47 | Lis | R |
| 58407.1705 | 58407.2318 | 15.535 | 0.011 | 56 | Ter | C |
| 58408.1950 | 58408.2035 | 16.669 | 0.058 | 5 | CRI | C |
| 58409.1758 | 58409.2163 | 17.180 | 0.029 | 36 | Ter | C |
| 58409.1802 | 58409.2329 | 17.080 | 0.023 | 74 | Lis | R |
| 58410.1569 | 58410.2130 | 17.037 | 0.017 | 48 | Ter | C |
| 58410.1749 | 58410.2102 | 17.050 | 0.026 | 50 | Lis | R |
| 58411.1742 | 58411.1827 | 17.111 | 0.105 | 5 | CRI | C |
| 58414.1673 | 58414.2055 | 15.041 | 0.011 | 54 | Lis | R |

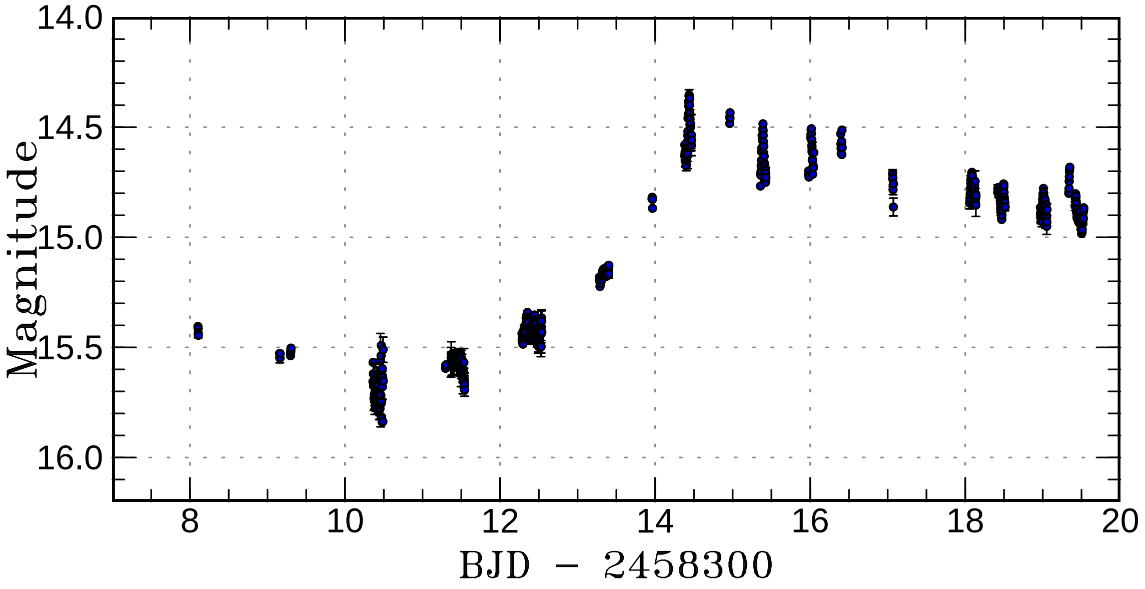


**E-figure 1.** The rise of SO2 from standstill. There was no hint of a precursor outburst or a “shoulder” as seen in Kepler observations of V1504 Cyg and V344 Lyr (Osaki and Kato 2013a; Osaki and Kato 2013b). The data were binned to 0.002 d.

**E-table 2.** Superhump maxima of NY Ser during SO1

| $E$ | max* | error | $O-C$† | $N$‡ |
|---|---|---|---|---|
| 0 | 58200.5622 | 0.0011 | 0.0079 | 79 |
| 6 | 58201.1773 | 0.0003 | 0.0018 | 205 |
| 7 | 58201.2744 | 0.0006 | −0.0046 | 207 |
| 9 | 58201.4858 | 0.0010 | −0.0003 | 209 |
| 16 | 58202.2147 | 0.0008 | 0.0040 | 217 |
| 17 | 58202.3159 | 0.0006 | 0.0016 | 84 |
| 18 | 58202.4194 | 0.0009 | 0.0017 | 210 |
| 19 | 58202.5241 | 0.0007 | 0.0028 | 143 |
| 20 | 58202.6257 | 0.0019 | 0.0009 | 36 |
| 26 | 58203.2428 | 0.0016 | −0.0031 | 76 |
| 27 | 58203.3607 | 0.0037 | 0.0112 | 145 |
| 28 | 58203.4498 | 0.0012 | −0.0032 | 165 |
| 31 | 58203.7575 | 0.0068 | −0.0061 | 39 |
| 32 | 58203.8697 | 0.0019 | 0.0026 | 67 |
| 35 | 58204.1766 | 0.0009 | −0.0011 | 110 |
| 36 | 58204.2815 | 0.0009 | 0.0003 | 111 |
| 45 | 58205.2154 | 0.0015 | 0.0025 | 111 |
| 46 | 58205.3218 | 0.0011 | 0.0054 | 77 |
| 54 | 58206.1471 | 0.0010 | 0.0025 | 115 |
| 66 | 58207.3741 | 0.0027 | −0.0128 | 104 |
| 67 | 58207.4991 | 0.0049 | 0.0086 | 104 |
| 74 | 58208.1856 | 0.0014 | −0.0295 | 111 |
| 75 | 58208.2973 | 0.0014 | −0.0213 | 141 |
| 84 | 58209.2431 | 0.0009 | −0.0072 | 111 |
| 86 | 58209.4575 | 0.0018 | 0.0001 | 36 |
| 112 | 58212.1656 | 0.0015 | 0.0166 | 94 |
| 113 | 58212.2713 | 0.0010 | 0.0188 | 111 |

*BJD−2400000.

†Against max $= 2458200.5544 + 0.103524E$.

‡Number of points used to determine the maximum.

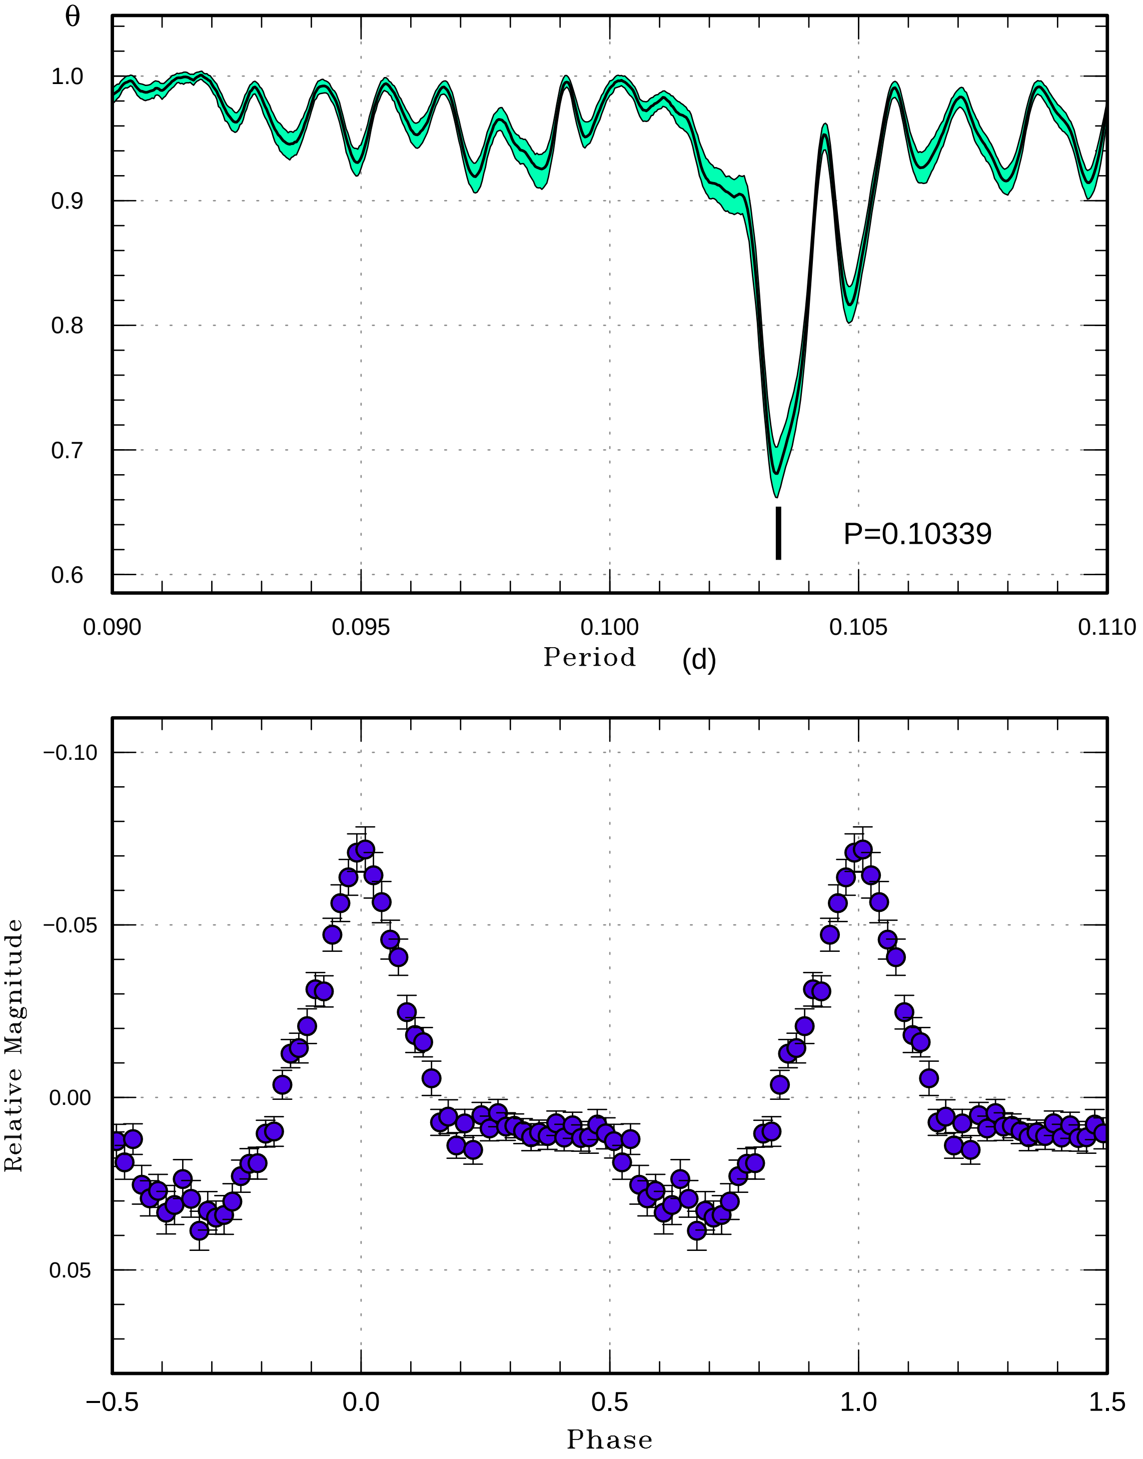


**E-figure 2.** Mean profile of superhumps in SO1. The data between BJD 2458200 and 2458210 were used. (Upper): PDM analysis. We analyzed 100 samples which randomly contain 50% of observations, and performed PDM analysis for these samples. The result is shown as a form of 90% confidence intervals in the resultant PDM $\theta$ statistics. The mean superhump period was 0.10339(1) d. (Lower): Phase-averaged profile.

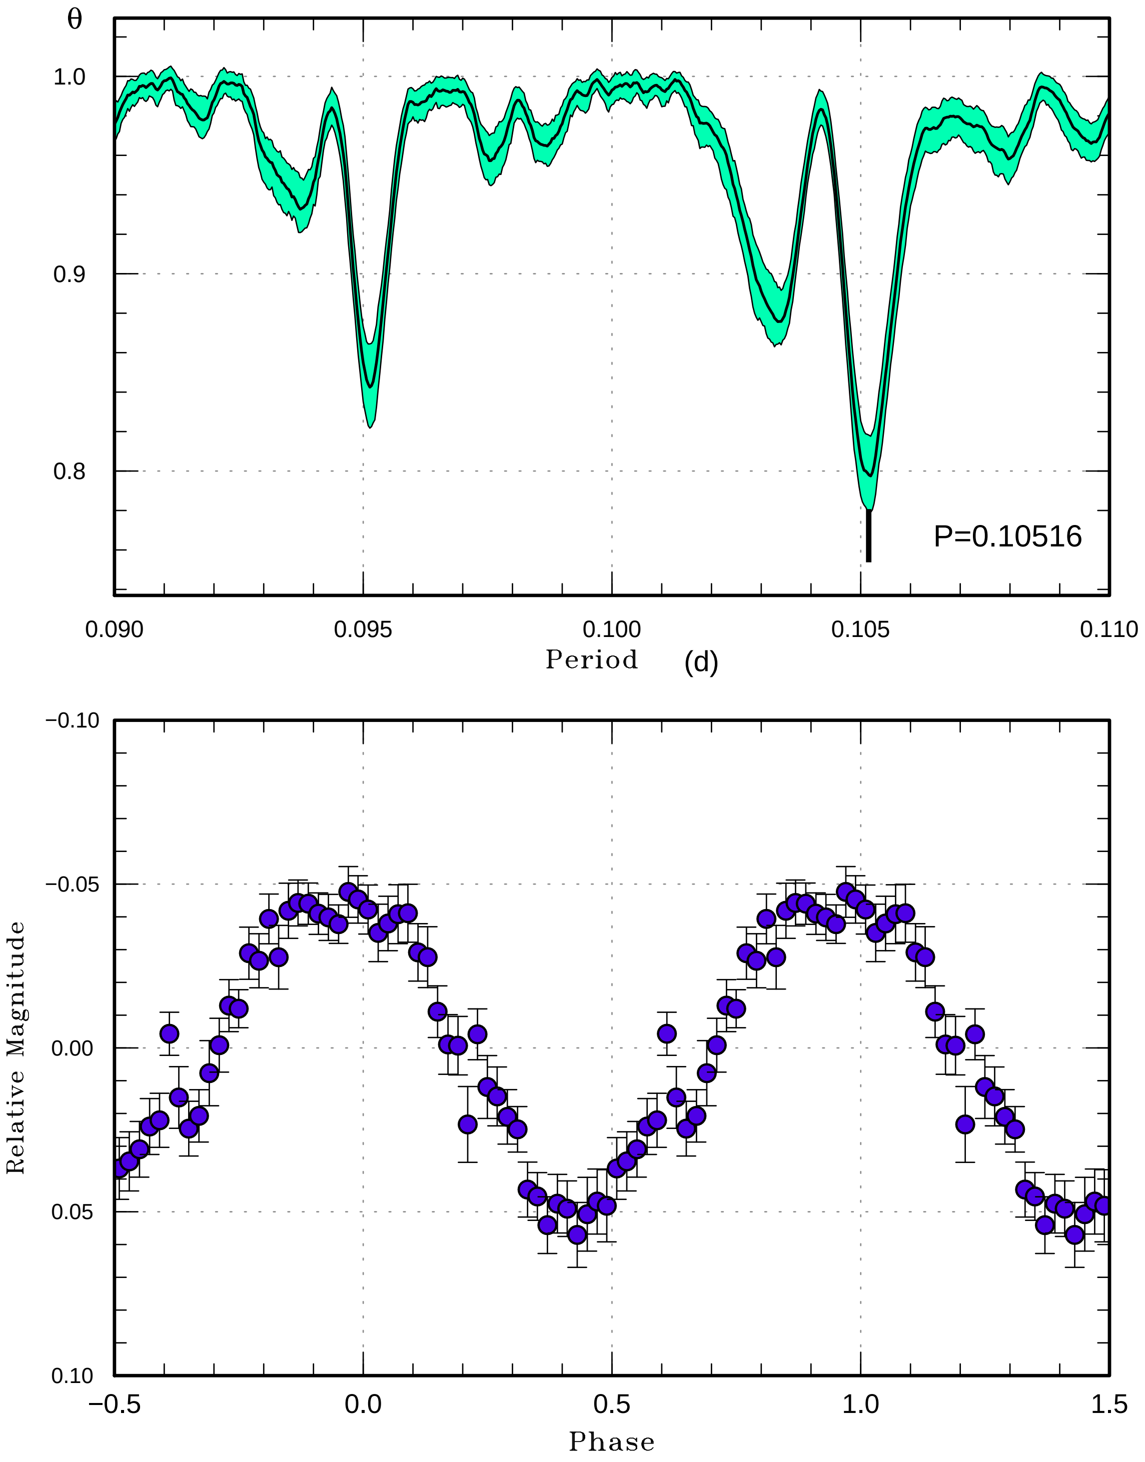


**E-figure 3.** Long-period superhumps after SO1. The data between BJD 2458213 and 2458222 were used. (Upper): PDM analysis. The mean superhump period was 0.10516(3) d. The signal near 0.095 d is its one-day alias. (Lower): Phase-averaged profile.

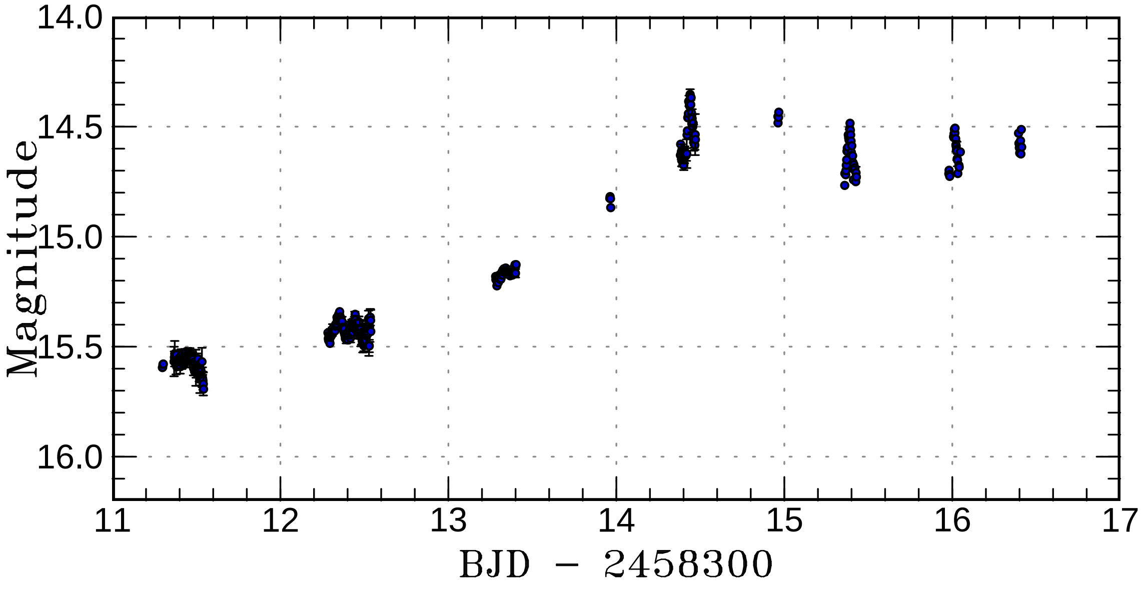


**E-figure 4.** Development of superhumps in the rising phase of SO2 in NY Ser. The data were binned to 0.002 d.

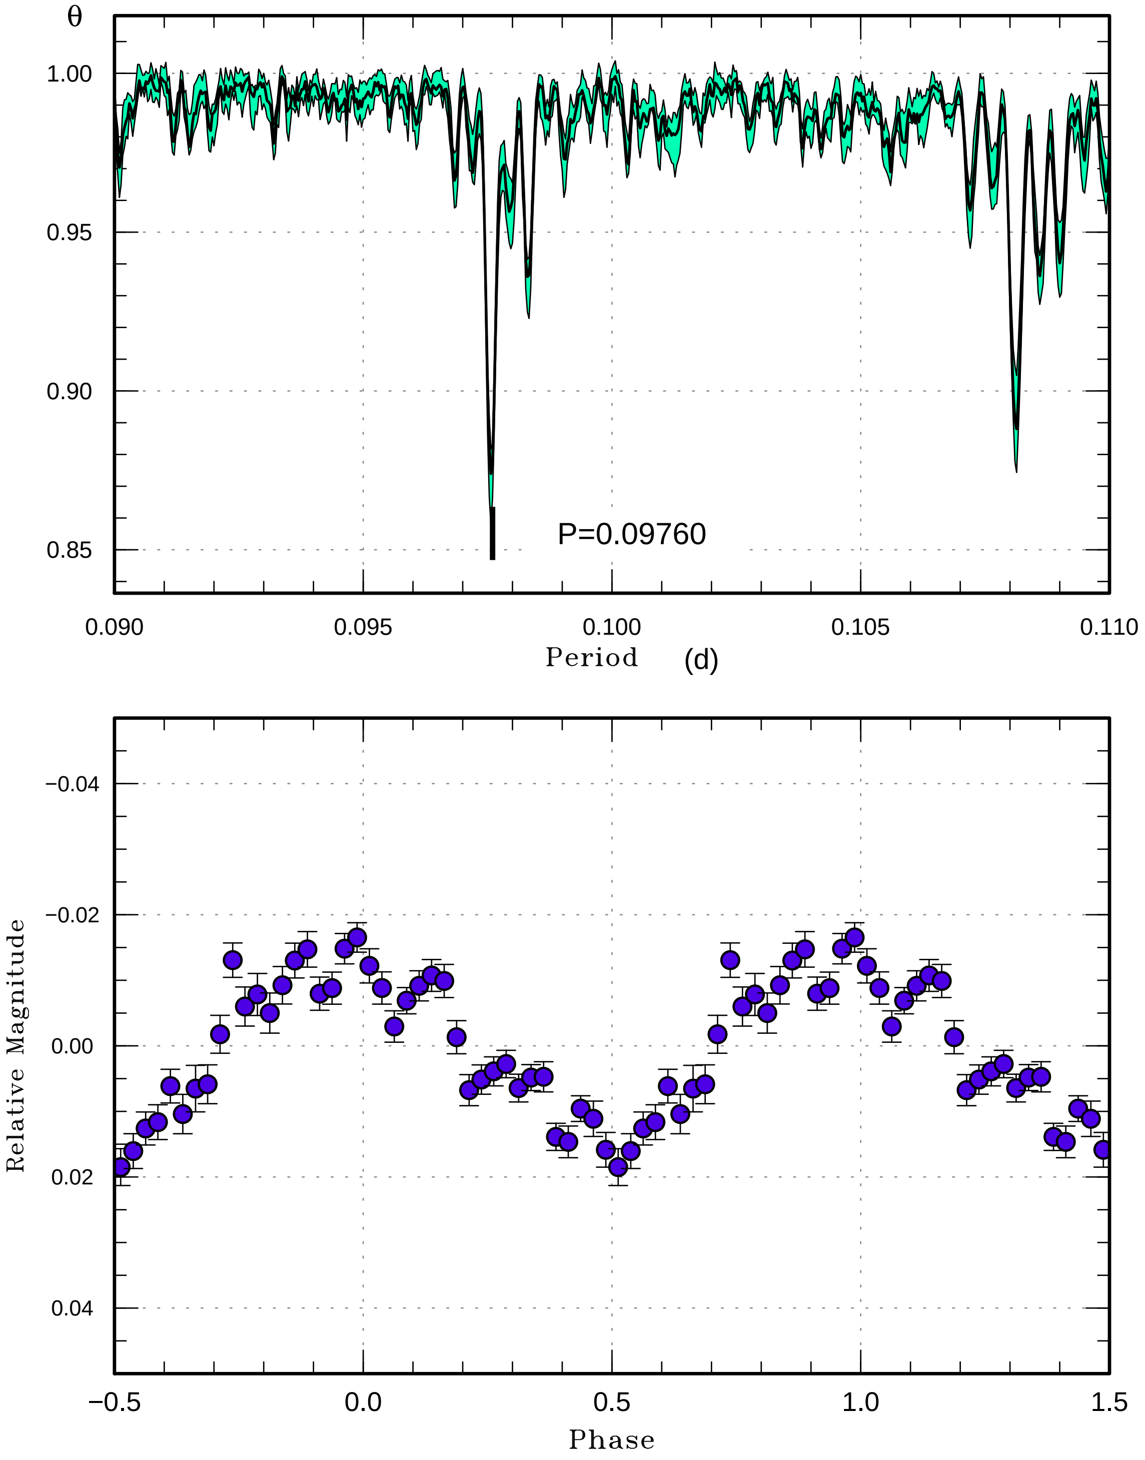


**E-figure 5.** Perid analysis during the second standstill. The data between BJD 2458261 and 2458306 were used. (Upper): PDM analysis. The only signal is the orbital one at 0.09760(3) d. The signal near 0.106 d is its one-day alias. (Lower): Phase-averaged profile.
